# Supplementary material for: NeRF-LiDAR: Generating Realistic LiDAR Point Clouds with Neural Radiance Fields
Source: arXiv:2304.14811 source file (2024-01-20)
Supplement: Supplementary file 1 [file supp_psnr_compare.tex]

\setlength{\tabcolsep}{20pt}

\begin{table}[ht!]
\vspace{-1mm}
\centering
\resizebox{1\linewidth}{!}{
\begin{tabular}{l|lll}
% &\multicolumn{3}{c|}{RGB metrics}  \\
\toprule
           & PSNR$\uparrow$ & SSIM $\uparrow$& LPIPS$\downarrow$ \\ \hline
NeRF-LiDAR &   \textbf{25.19 }  &  \textbf{0.802 }   &   \textbf{0.328}  \\ 
 %PNF\\
 Urban-NeRF ~\cite{urban-nerf} &21.12&	0.673	&0.503 \\
%\hline
           % &      &      &       &               &       
           \bottomrule
\end{tabular}
}
\vspace{1mm}
\caption{Evaluation of NeRF-LiDAR and Urban-NeRF using RGB metrics in the reconstructed scenes.}% Error rate∗\text{Error rate}^* means the percentage which of relative error exceeds 10%10\%}.
\label{tab:nerf_lidar_eva}
\end{table}
